# Supplementary material for: Graph AI generates neurological hypotheses validated in molecular, organoid, and clinical systems
Source: arXiv:2512.13724 ancillary file (2025-12-13)
Supplement: Supplementary file 1 [file PROTON_SI.pdf]

# Supplementary Information for Graph AI generates hypotheses validated across neurological systems

Ayush Noori[1,2,3,4,5,6,7], Joaquín Polonuer[1], Katharina Meyer[2,5,8], Bogdan Budnik[2,5], Shad Morton[2,5], Xinyuan Wang[6,9], Sumaiya Nazeen[6,9], Yingnan He[3], Iñaki Arango[1], Lucas Vittor[1], Matthew Woodworth[2,5,8], Richard C. Krolewski[6,9], Michelle M. Li[1,6], Ninning Liu[2,5], Tushar Kamath[10], Evan Macosko[10], Dylan Ritter[6,11], Jalwa Afroz[6,11], Alexander B. H. Henderson[3,6], Lorenz Studer[6,11], Samuel G. Rodriques[12], Andrew White[12], Noa Dagan[7,13,14], David A. Clifton[4,15], George M. Church[2,5,8], Sudeshna Das[3,†], Jenny M. Tam[2,5,8,†], Vikram Khurana[6,9,10,16,†], Marinka Zitnik[1,6,7,10,17,18,†]

[1]Department of Biomedical Informatics, Harvard Medical School, Boston, MA, USA
[2]Wyss Institute for Biologically Inspired Engineering at Harvard University, Boston, MA, USA
[3]Department of Neurology, Massachusetts General Hospital, Boston, MA, USA
[4]Department of Engineering Science, University of Oxford, Oxford, UK
[5]BD$^2$: Breakthrough Discoveries for thriving with Bipolar Disorder, Santa Monica, CA, USA
[6]Aligning Science Across Parkinson's (ASAP) Collaborative Research Network, Chevy Chase, MD, USA
[7]The Ivan and Francesca Berkowitz Family Living Laboratory Collaboration at Harvard Medical School and Clalit Research Institute, Boston, MA, USA
[8]Department of Genetics, Harvard Medical School, Boston, MA, USA
[9]Department of Neurology, Brigham and Women's Hospital, Boston, MA, USA
[10]Broad Institute of MIT and Harvard, Cambridge, MA, USA
[11]The Center for Stem Cell Biology, Memorial Sloan Kettering Cancer Center, New York, NY, USA
[12]FutureHouse Inc., San Francisco, CA, USA
[13]Clalit Research Institute, Innovation Division, Clalit Health Services, Ramat-Gan, Israel
[14]Faculty of Computer and Information Science, Ben Gurion University of the Negev, Be'er Sheva, Israel
[15]Oxford Suzhou Centre for Advanced Research, University of Oxford, Suzhou, Jiangsu, China
[16]Harvard Stem Cell Institute, Cambridge, MA, USA
[17]Kempner Institute for the Study of Natural and Artificial Intelligence, Harvard University, MA, USA
[18]Harvard Data Science Initiative, Cambridge, MA, USA

[†]Correspondence: sdas5@mgh.harvard.edu, jenny.tam@wyss.harvard.edu, vkhurana@bwh.harvard.edu, marinka@hms.harvard.edu (lead contact)

PROTON website: https://protonmodel.ai
PROTON code: http://github.com/mims-harvard/PROTON
PROTON model: https://huggingface.co/mims-harvard/PROTON

**This PDF file includes:**

Supplementary Notes 1 to 5

Supplementary Figures 1 to 8

Supplementary Tables 1 to 5

# Supplementary Note 1: PROTON embeddings are biomedically organized

The learned embedding space of PROTON was visualized using the uniform manifold approximation and projection algorithm (UMAP) for non-linear dimensionality reduction [1, 2] implemented in the `scikit-learn` machine learning library [3]. We used a cosine similarity distance function, a local neighborhood size of 15, and a minimum distance of 0.8; however, UMAP results were largely invariant to these hyperparameter choices. Clustering was observed by node type identity – that is, nodes with the same biomedical identity occupied similar regions of the embedding space – suggesting that PROTON effectively projects NEUROKG into a meaningful learned latent space (Supplementary Figure 1).

## 1.1 Related diseases cluster together in the PROTON latent space

To further evaluate PROTON embeddings, we examined disease nodes. MONDO disease terms were grouped into four categories based on their hierarchical position in the MONDO disease ontology [4, 5]: neurodegenerative diseases (descendants of `MONDO:0005559`, $n = 772$), cancers (descendants of `MONDO:000499`, $n = 2,208$), infectious diseases (descendants of `MONDO:0005550`, $n = 1,060$), and an "other" category for all remaining diseases. Diseases classified under multiple parent categories were assigned to "other," resulting in 750 neurodegenerative diseases, 2,198 cancers, and 1,028 infectious diseases. The disease nodes in NEUROKG corresponding to these MONDO disease terms formed four subgraphs: 693 neurodegenerative diseases, 982 infectious diseases, 2,117 cancers, and 18,409 other diseases.

The PROTON disease embedding space was visualized using cosine-similarity-based UMAP (with the same parameters as above), which revealed that neurodegenerative diseases segregate from cancers and infectious diseases in the PROTON latent space (Supplementary Figure 2a). To quantitatively assess this separation based on distance in the high-dimensional embedding space – rather than in the low-dimensional UMAP projection, which may not preserve distances or structure [6] – we computed the silhouette coefficient for each disease node:

$$S(u) = \frac{b(u) - a(u)}{\max(a(u), b(u))}$$

where $a$ is the mean intra-cluster distance and $b$ is the mean nearest-cluster distance:

$$a(u) = \frac{1}{|C_u| - 1} \sum_{v \in C_u, v \neq u} \text{dist}(u, v)$$

$$b(u) = \min_{C_k \neq C_u} \left( \frac{1}{|C_k|} \sum_{v \in C_k} \text{dist}(u, v) \right)$$

Here, $C_u$ represents the set of diseases in the same cluster as $u$, $|C_u|$ is its cardinality, and $\text{dist}(u, v)$ is the cosine-similarity-based distance between diseases $u$ and $v$, given by:

$$\text{dist}(u, v) = 1 - \frac{\mathbf{x}_u \cdot \mathbf{x}_v}{|\mathbf{x}_u||\mathbf{x}_v|}$$

which is scaled to the $[0, 1]$ range using min-max normalization. The term $b(u)$ is computed by taking the minimum average distance over all clusters $C_k$ to which $u$ does not belong. Finally, the silhouette coefficient for each cluster was determined by averaging over all constituent diseases.

The silhouette coefficient ranges from $[-1, 1]$, where 1 indicates well-separated clusters (*e.g.*, perfect clusters in synthetic data), 0 suggests overlapping clusters, and negative values imply potential misclassifications since a disease is closer to another cluster than its assigned one. As shown in Supplementary

Figure 2b, neurodegenerative diseases possess the highest silhouette score (0.1847), followed by cancers (0.1331) and then infectious diseases (0.0255). Diseases not assigned to a specific category have a negative score (−0.1951), suggesting they lack clear separation relative to the three selected categories. These results demonstrate that PROTON capably organizes diseases into broad medical categories in its learned embedding space.

### 1.2 Structurally-similar drugs cluster in the PROTON latent space

Next, we examined drug representations learned by PROTON. We first sought to identify groupings of drugs in NEUROKG by structural similarity. For each drug node in NEUROKG, the corresponding chemical structure was retrieved in the simplified molecular-input line-entry system (SMILES) format [7]. Isomeric SMILES structures with isotopic and chiral specifications were obtained by querying the PubChem [8] application programming interface (API) with DrugBank identifiers [9]. Using RDKit [10], an open-source cheminformatics toolkit, the SMILES representations of all drugs were converted to molecular graphs, where nodes correspond to atoms and edges correspond to chemical bonds. Based on the molecular graphs, we then created molecular fingerprints, or vector representations of the structural properties of each molecule, which encode the local chemical environment of a molecule by iteratively applying a hashing function to molecular substructures [11]. In particular, we use the Morgan fingerprint, a 2048-bit vector where bits are assigned based on the presence of circular substructures around each atom in a molecule [12]. We use a radius of 2; therefore, the hashing function is applied to all substructures within 2 bonds of each atom in the molecule. Of the 8,160 drugs in NEUROKG, SMILES structures were available, molecular graphs were created, and Morgan fingerprints were computed for 6,943 drugs (85.09%).

Next, for all drugs with Morgan fingerprints, the pairwise Tanimoto similarity was computed and converted to a distance metric with $\text{dist}(d_1, d_2) = 1 - \text{Tanimoto}(d_1, d_2)$. Finally, drugs were grouped into structurally similar clusters by agglomerative hierarchical clustering with the average distance linkage criterion and a distance threshold of 0.8. A total of 847 clusters were identified, from which the 20 largest clusters containing at least 55 molecules were analyzed. Altogether, these 20 clusters encompassed 1,844 drugs; the remaining 5,099 drugs were assigned a cluster of "other." The pharmacological similarities uniting drug clusters were interpreted by querying GPT-4o [13] with the constituent drugs of each cluster, along with the prompt, "What do these drugs have in common?" Based on model responses, selected clusters of interest were manually assigned human-readable labels.

The PROTON drug embedding space was visualized using cosine-similarity-based UMAP (with the same parameters as above), which revealed that drugs segregate by structural similarity in the PROTON learned embedding space (Supplementary Figure 3). The embedding-based silhouette scores of the 20 largest clusters relative to each other and to the outgroup of 5,099 uncategorized drugs are shown in Supplementary Figure 3b. Selected clusters of interest are highlighted in the drug embedding UMAP in Supplementary Figure 3a and with colored bars in Supplementary Figure 3b.

The largest cluster, Cluster 1 (with a cluster-wide mean silhouette score of 0.2359), contained 250 nucleoside or nucleotide analogs, including reverse transcriptase inhibitors used to treat HIV/AIDS, herpes viruses, and hepatitis B virus; antimetabolite chemotherapeutic agents; and nucleotide derivatives involved in cellular metabolism. Cluster 4 (0.2076) contained 126 steroids, including glucocorticoids, mineralocorticoids, progestins, androgens, antiandrogens, and anabolic steroids. Cluster 9 (0.0902) contained 79 additional steroid hormones and hormone analogs, including estrogens, progestins, and androgens. Given that clusters 4 and 9 both contain steroid hormones, the overlap between these clusters in the latent space is encouraging (Supplementary Figure 3a). Cluster 12 (0.1303) was composed of phosphate-containing molecules primarily involved in metabolism, nucleotide biosynthesis, and cellular signaling, including

phosphorylated sugars and carbohydrates involved in glycolysis, gluconeogenesis, and pentose phosphate pathways; phosphate-linked nucleosides; inositol phosphates; phospholipids; and organophosphates. Cluster 16 (0.2191) contained 61 benzimidazole-based compounds that impede tubulin polymerization with antiparasitic, antifungal, or microtubule-disrupting properties. Cluster 17 (0.3344) contained 58 cephalosporins and related $\beta$-lactam antibiotics that inhibit bacterial cell wall synthesis. Cluster 18 (0.1211) contained 57 drugs that modulate neurotransmitter systems, including anticholinergics, opioids and opioid-like compounds, and antihistamines. Finally, Cluster 20 (0.0905) contained 55 drugs that share a sulfonamide functional group, including selective cyclooxygenase-2 inhibitors, sulfonamide-based antiepileptics, and antibacterial sulfonamides. By contrast, the group of 5,099 uncategorized drugs had a silhouette score of −0.1586, suggesting that they lack clear separation relative to the top 20 largest drug categories.

Of note, Proton was never provided with molecular structure during pre-training; rather, Proton was trained on the interactome of each drug represented in NeuroKG. Nonetheless, this analysis indicates that Proton can recover the structural organization of drugs purely from their interaction networks. Given that structurally similar drugs often share similar pharmacological properties, these findings suggest that Proton captures functionally relevant features beyond what is explicitly provided in the training data.

# Supplementary Note 2: An AI agent validates disease edges in NeuroKG

We sought to evaluate whether edges in NeuroKG are high-quality and supported by evidence in the scientific literature. To do so, we used PaperQA2, a frontier language-based generative AI agent that retrieves and reasons on information from the scientific literature [14, 15]. PaperQA2 answers user questions by performing multi-step literature-grounded retrieval-augmented generation (RAG) [16] using four tools: "Paper Search," which identifies, parses, and embeds candidate scientific papers from keywords in the user query; "Gather Evidence," which injects summaries of relevant papers identified by top-$k$ dense vector retrieval, LLM reranking, and contextual summarization steps; "Citations Traversal," which adds additional sources from the citation graph; and "Generate Answer," which produces a final answer. Among the databases that PaperQA2 can retrieve papers from include arXiv, medRxiv, bioRxiv, ChemRxiv, PubMed, PubMed Central, and open-access papers.

We selected six neurological diseases and, for each disease, queried NeuroKG for all edges of type `(disease, disease)`, `(disease, gene/protein)`, `(disease, drug)`, or `(disease, exposure)` in the neighborhood of that disease. There were 433 edges incident on amyotrophic lateral sclerosis, 648 edges incident on epilepsy, 1,033 edges incident on multiple sclerosis, 1,072 edges incident on Parkinson's disease, 685 edges incident on bipolar disorder, and 326 edges incident on major depressive disorder, for a total of 4,197 edges. For each edge, we tasked PaperQA2 with evaluating whether that association is supported by evidence in the scientific or medical literature. Specifically, PaperQA2 was prompted to assign an integer score from 1 to 5 for each edge, where 1 indicates no supporting evidence found, 2 indicates weak evidence, with 1-2 papers in support; 3 indicates moderate evidence, with 3-4 papers in support; 4 indicates strong evidence, with 5-6 papers in support; and 5 indicates very strong evidence, with over 6 supporting papers or substantial experimental evidence. For each response, PaperQA2 also provided reasoning behind each rating and referenced scientific or medical sources to support its assessment, including peer-reviewed studies, clinical guidelines, or experimental data retrieved via API calls to the Open Targets platform. As a negative control, PaperQA2 was also tasked with evaluating 100 random non-edges for each disease (*i.e.*, associations between each disease and 100 randomly selected nodes of type `disease`, `gene/protein`, `drug`, or `exposure`), using the same prompt and instructions. PaperQA2 generated structured responses in eXtensible Markup Language (XML).

The LLM used for answer generation and contextual summarization was Claude 3.5 Sonnet (version `20241022`) from Anthropic, while the `text-embedding-3-large` model from OpenAI was used to generate embedding vectors of parsed paper sections. PaperQA2 was queried using the `pqapi` package (version 7.2.0) in Python (version 3.11.10). From a total of 4,797 queries to PaperQA2, the AI agent could not generate an answer for 13 responses, six of which were negative control queries. Among the successful experimental queries, for each query and response, PaperQA2 parsed and reviewed an average of $14.50 \pm 5.75$ (mean ± SD, $n = 4,197$) papers, cited average $5.43 \pm 1.79$ references in the final answer, and required average $140.48 \pm 81.99$ seconds to generate a response at an average cost of \$0.26 ± 0.09 per query.

PaperQA2 identified scientific evidence to support 83.87% of edges ($n = 3,514$) (Supplementary Figure 6). Of those edges, 35.37% were weakly supported (*i.e.*, 1-2 papers, $n = 1,243$), 28.03% were moderately supported (*i.e.*, 3-4 papers, $n = 985$), 12.64% were strongly supported (*i.e.*, 5-6 papers, $n = 444$), and 23.96% were very strongly supported (*i.e.*, greater than 6 papers, $n = 842$). Only 16.13% of edges were not supported by any evidence ($n = 676$); of these, the majority were gene-disease associations, which is expected, as many gene-disease associations were derived directly from experimental evidence from the Open Targets Platform or other sources and may not yet be supported by published papers in the scientific literature. By contrast, for the negative control of random non-edges, 75.54% ($n = 448$) of non-edges were not supported by any evidence, and only 1.85% ($n = 11$) of edges were very strongly supported. These results suggest that, across several neurological diseases, associations in NeuroKG are high-quality, factual, and can be supported by the scientific and medical literature.

## Supplementary Note 3: NeuroKG encompasses nervous system entities

NeuroKG offers broad coverage of biomedical entities in the human nervous system across health and disease. For example, according to the Human Protein Atlas (HPA), 16,465 human protein-coding genes are expressed in the brain, based on the highest expression value of the gene detected across 13 brain regions, the spinal cord, and the corpus callosum [17]. Of those, 16,089 genes, or 97.72%, are represented in NeuroKG. Similarly, of the 3,195 neuroanatomical entities included within the neurological (*i.e.*, “nervous-minimal”) subset of the Uberon integrated anatomical ontology [18, 19], 2,938 entities, or 91.96%, are represented in NeuroKG. Finally, of the 5,554 neurological diseases that are descendants of the “nervous system disorder” term (`MONDO:0005071`) in the MONDO disease ontology [4, 5], 5,130 diseases, or 92.37%, are represented in NeuroKG. Altogether, the coverage of neuroanatomical features, brain-expressed genes, and neurological diseases suggests that NeuroKG may be a valuable resource for research into the human nervous system.

## Supplementary Note 4: NeuroKG is more comprehensive than current KGs

Even with the stringent filtering steps taken during its construction, NeuroKG is more comprehensive than other state-of-the-art biomedical KGs. For example, PrimeKG has 129,375 nodes and 4,050,249 edges across 10 node types and 30 edge types [20]; `ogbl-biokg` has 93,773 nodes and 5,088,434 edges [21]; Hetionet features only 47,031 nodes and 2,250,197 edges across 11 node types and 24 edge types [22]; PharmKG has 7,603 nodes and 500,958 edges [23]; DRKG has 97,238 nodes and 5,874,261 edges; and AlzKB has 118,902 nodes and 1,309,527 edges [24]. By the numbers of nodes, edges, and databases considered, these graphs all contain less information than NeuroKG. For instance, when compared to PrimeKG, which shares a similar graph construction methodology as NeuroKG, 8,038 genes exist in NeuroKG but not in PrimeKG, while only 511 genes exist in PrimeKG but not in NeuroKG. These differences are driven by increased coverage of

both coding and non-coding genes: NeuroKG features 1,913 microRNAs, 2,063 long intergenic non-protein coding RNAs, and various pseudogenes. Further, NeuroKG is unique in integrating scRNA-seq data at subcluster resolution, enabling patient single-cell data analyses.

## Supplementary Note 5: Proton makes consistent predictions across related diseases

We also assessed whether Proton's predictions are consistent across clinically related diseases. We reasoned that a drug relevant to one disease should be similarly prioritized for related conditions. To evaluate this, we used Proton (trained on the full NeuroKG graph) to generate therapeutic predictions across 25 neurological diseases and all 8,160 drugs; then, we computed pairwise Spearman rank correlations across disease pairs. To exclude consistently low-ranked drugs that may be poorly annotated or not relevant to neurological disease, we focused on the 3,071 drugs that appear at rank $\leq 2,000$ in at least one of the 25 evaluation diseases. Diseases were grouped into five categories: neurodegenerative, neuropsychiatric, neuroinfectious, neurological cancer, and other. Encouragingly, Proton indeed makes similar predictions for related diseases (Supplementary Figure 8a). Brain cancers – including oligodendroglioma, medulloblastoma, astrocytoma, ependymoma, craniopharyngioma, and meningioma – had strong intragroup and low intergroup correlation. Similarly, neuroinfectious diseases, including meningitis, neurosyphilis, and encephalitis, are clustered tightly. Interestingly, neuropsychiatric conditions – such as anxiety, autism spectrum disorder, attention deficit hyperactivity disorder (ADHD), schizophrenia, and bipolar disorder – clustered alongside neurodegenerative diseases, suggesting overlapping pharmacological profiles captured by Proton. This is consistent with clinical observations: behavioral and neuropsychiatric symptoms are prevalent in neurodegenerative disorders like Alzheimer's disease [25] and Parkinson's [26] disease. Further, several drugs originally developed for neuropsychiatric disease – including brexpiprazole (approved for schizophrenia), escitalopram (approved for major depression), methylphenidate (approved for ADHD), and lithium (approved for BD) – are in phase II or phase III clinical trials for Alzheimer's disease [27].

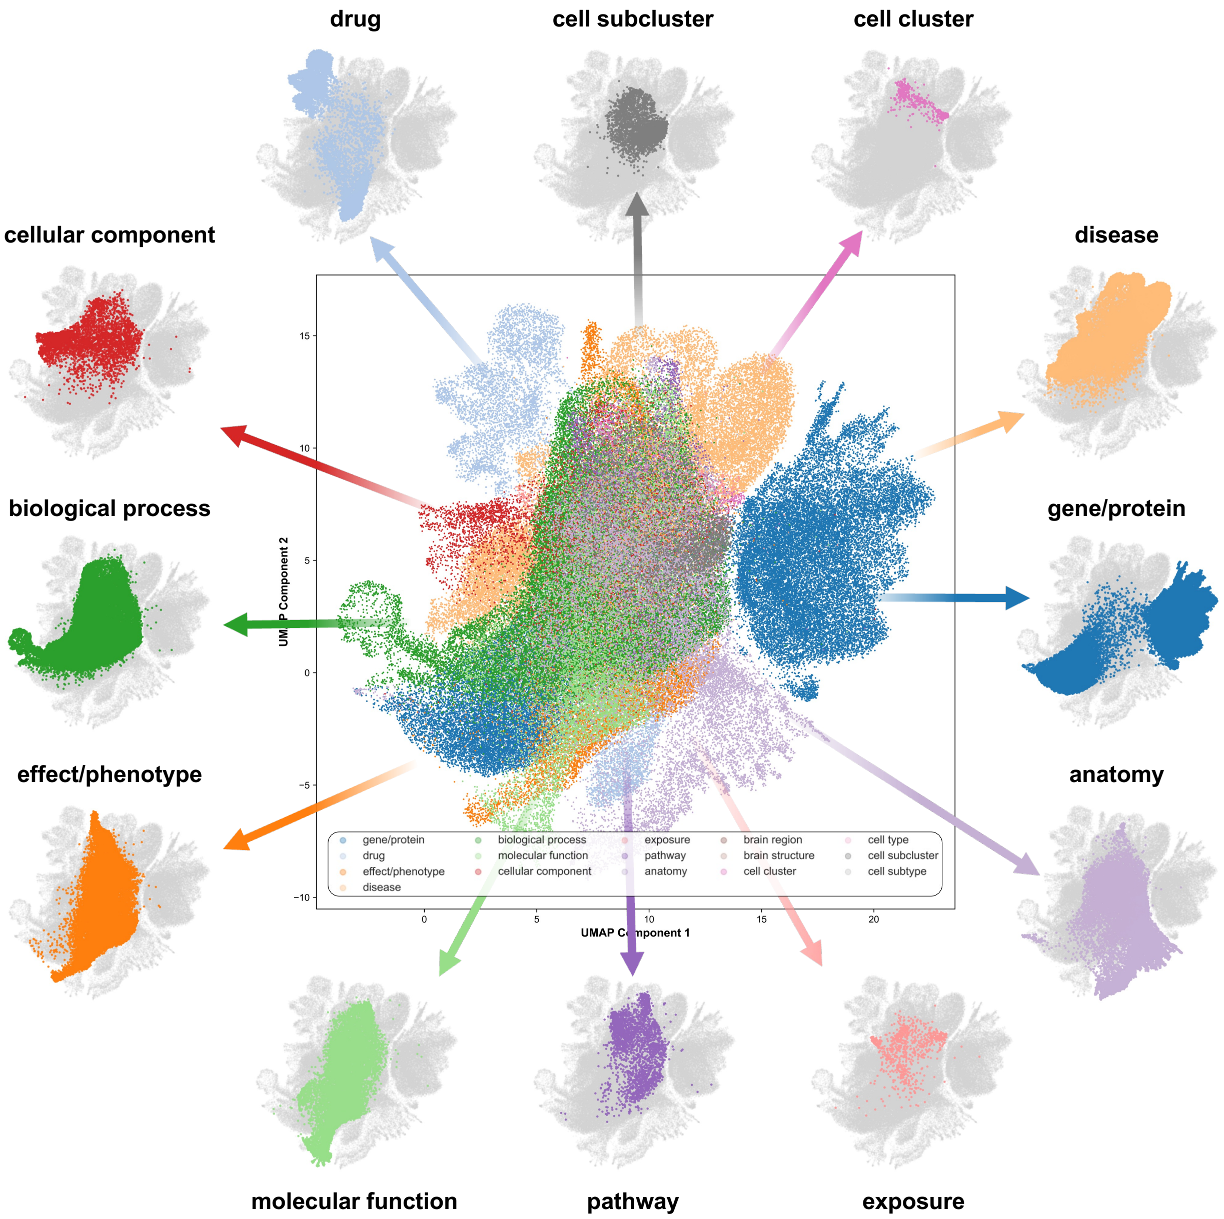


**Supplementary Figure 1: Proton embeddings are organized by biomedical identities and relationships.** The learned embedding space of Proton was visualized using the UMAP algorithm for non-linear dimensionality reduction. Nodes clustered based on their biomedical identity, suggesting that Proton successfully maps NeuroKG into a structured and meaningful latent representation.

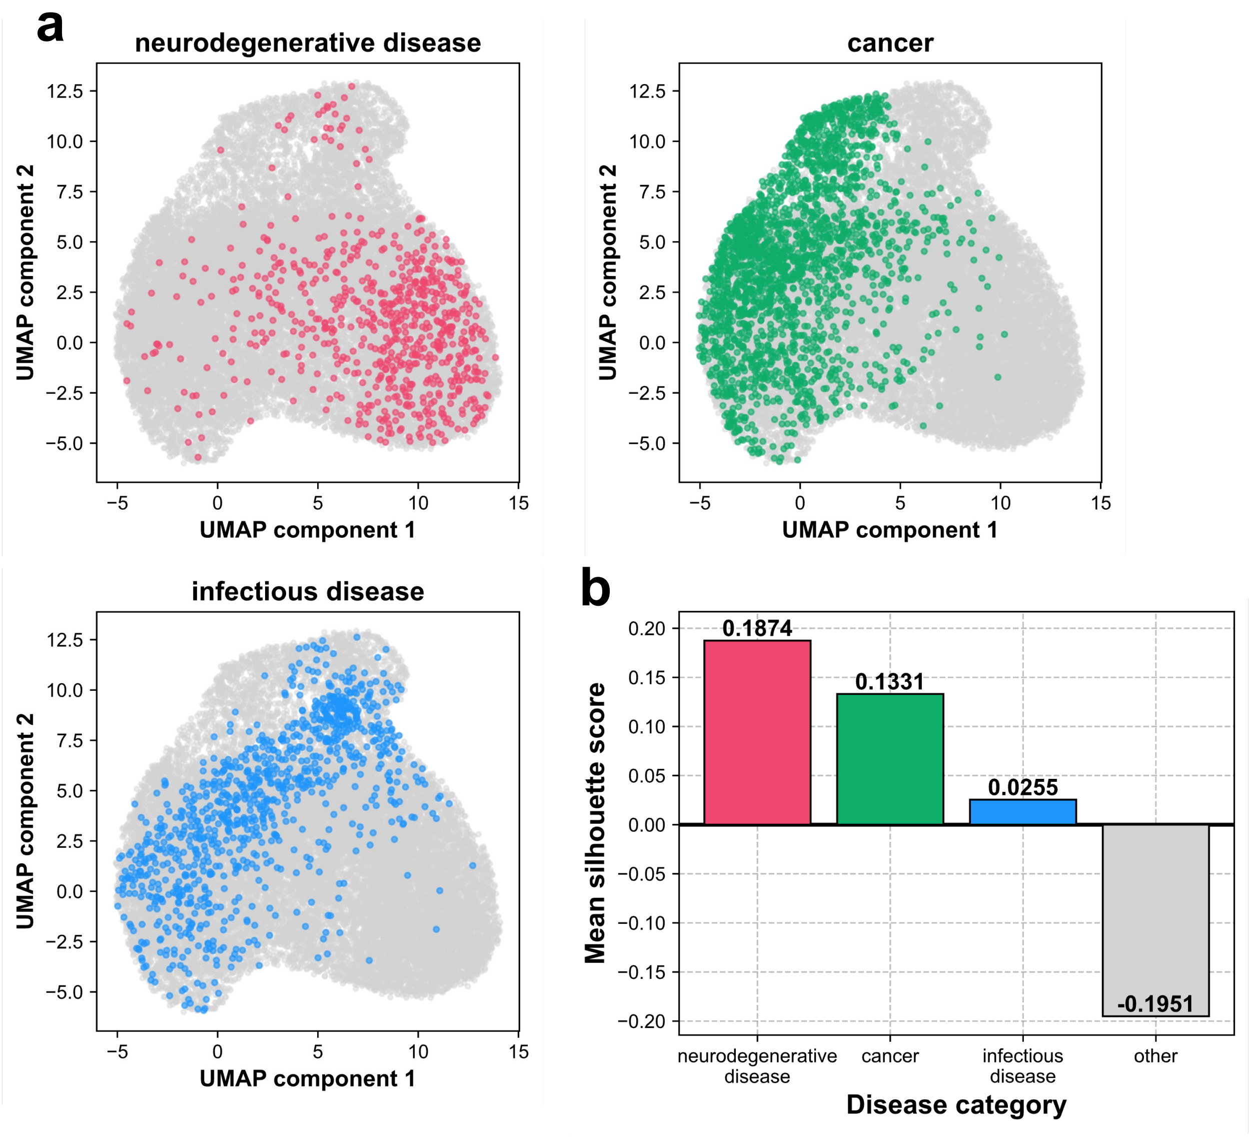


**Supplementary Figure 2: Related diseases cluster together in the learned PROTON latent space. (a)** A UMAP projection of disease embeddings based on cosine similarity shows that neurodegenerative diseases (red) segregate from cancers (green) and infectious diseases (blue) relative to all other diseases (gray). **(b)** Silhouette scores quantify the degree of separation between disease categories in the high-dimensional embedding space. Note that the separation between the three disease groups is relative to the fourth group of uncategorized diseases.

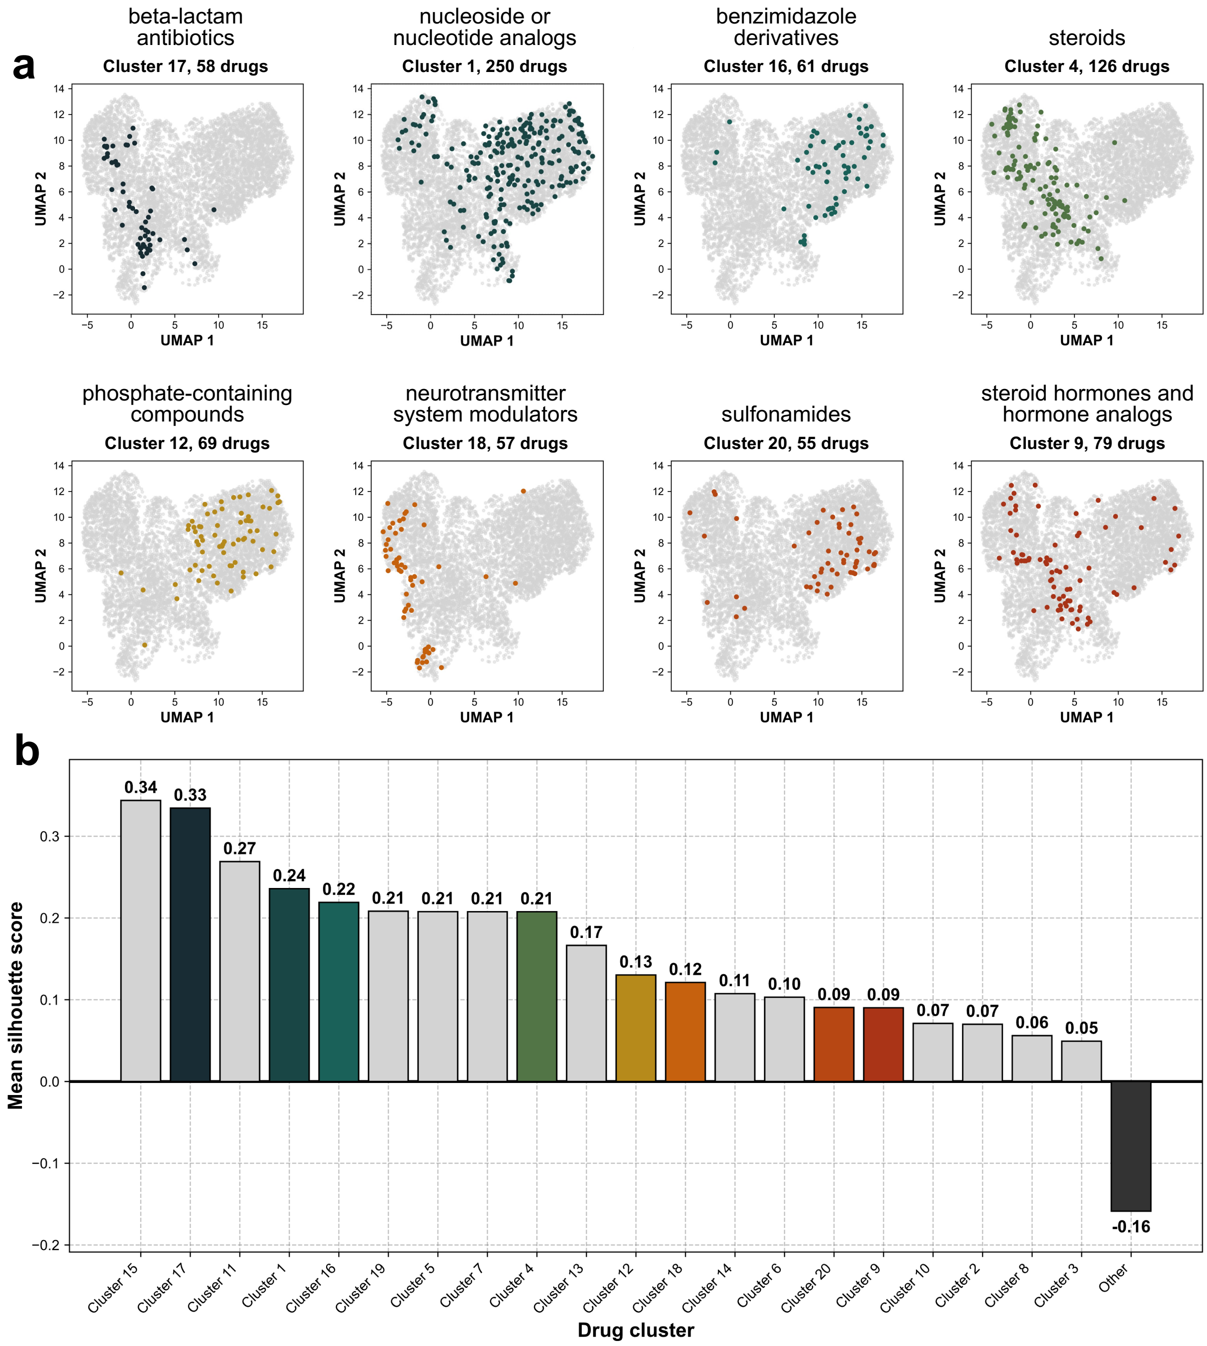


**Supplementary Figure 3: Structurally-similar drugs cluster together in the learned PROTON latent space. (a)** A UMAP projection of drug embeddings based on cosine similarity shows that drugs are grouped by structural and functional similarity. Colored points belong to the selected cluster, while gray points do not. **(b)** Silhouette scores quantify the degree of separation between drug categories in the high-dimensional embedding space. Note that the separation between the 20 largest clusters (containing a total of 1,844 drugs) is relative to the outgroup of 5,099 uncategorized drugs. Colored bars correspond to selected clusters of interest highlighted in panel (a).

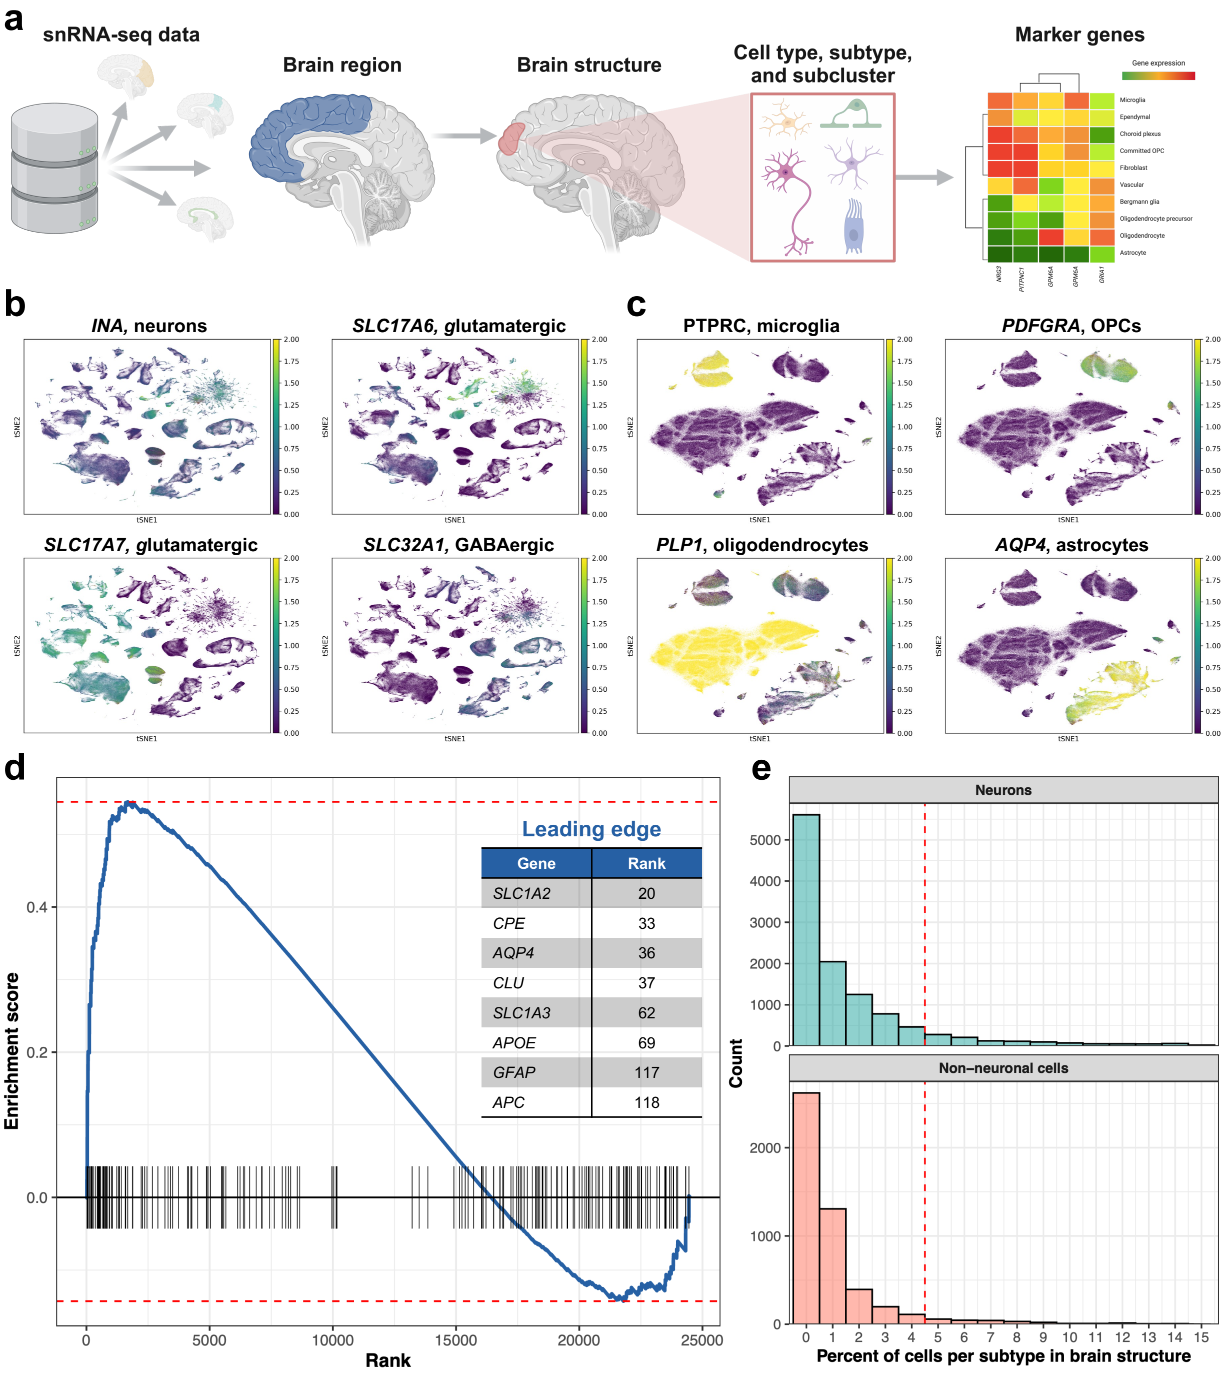


**Supplementary Figure 4: Analysis of 2,480,956 neurons and 888,263 non-neuronal cells integrated into NeuroKG.** **(a)** Structure of snRNA-seq derived edges in NeuroKG. Edges were constructed between brain regions, brain structures, cell types, cell subtypes, cell subclusters, and marker genes. **(b)** Neuronal and **(c)** non-neuronal cell types identified by Siletti *et al.* express known cell type-specific markers. See Figure 1 of Siletti *et al.* [28] for reference. **(d)** Astrocyte marker genes are significantly enriched for known immunohistochemical markers of astrocytes under gene set enrichment analysis ($p = 1.612 \times 10^{-4}$, ES = 0.545, NES = 1.623). **(e)** Proportions of cells of each subtype present per each brain structure. Most brain structures contain less than 5% of each subtype.

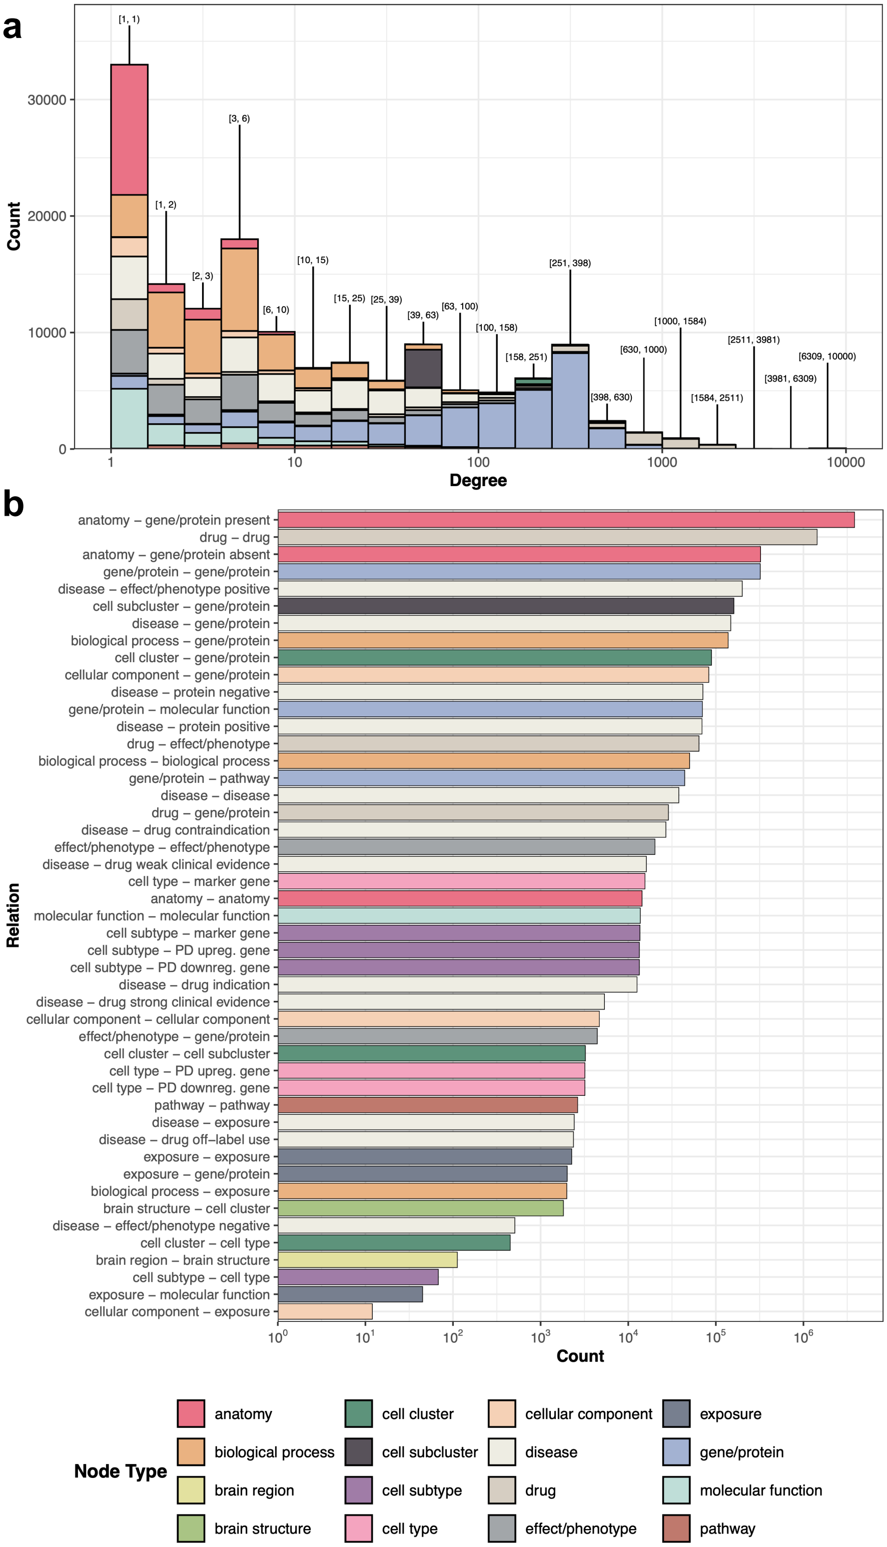


**Supplementary Figure 5: NeuroKG is a knowledge graph with 147,020 nodes and 7,366,745 edges.** **(a)** Distribution of degree by node type, see also Supplementary Table 2. **(b)** Number of edges per edge type. Bars are colored by the type of the tail node. Note that the $x$-axes of both panels are in logarithmic scale.

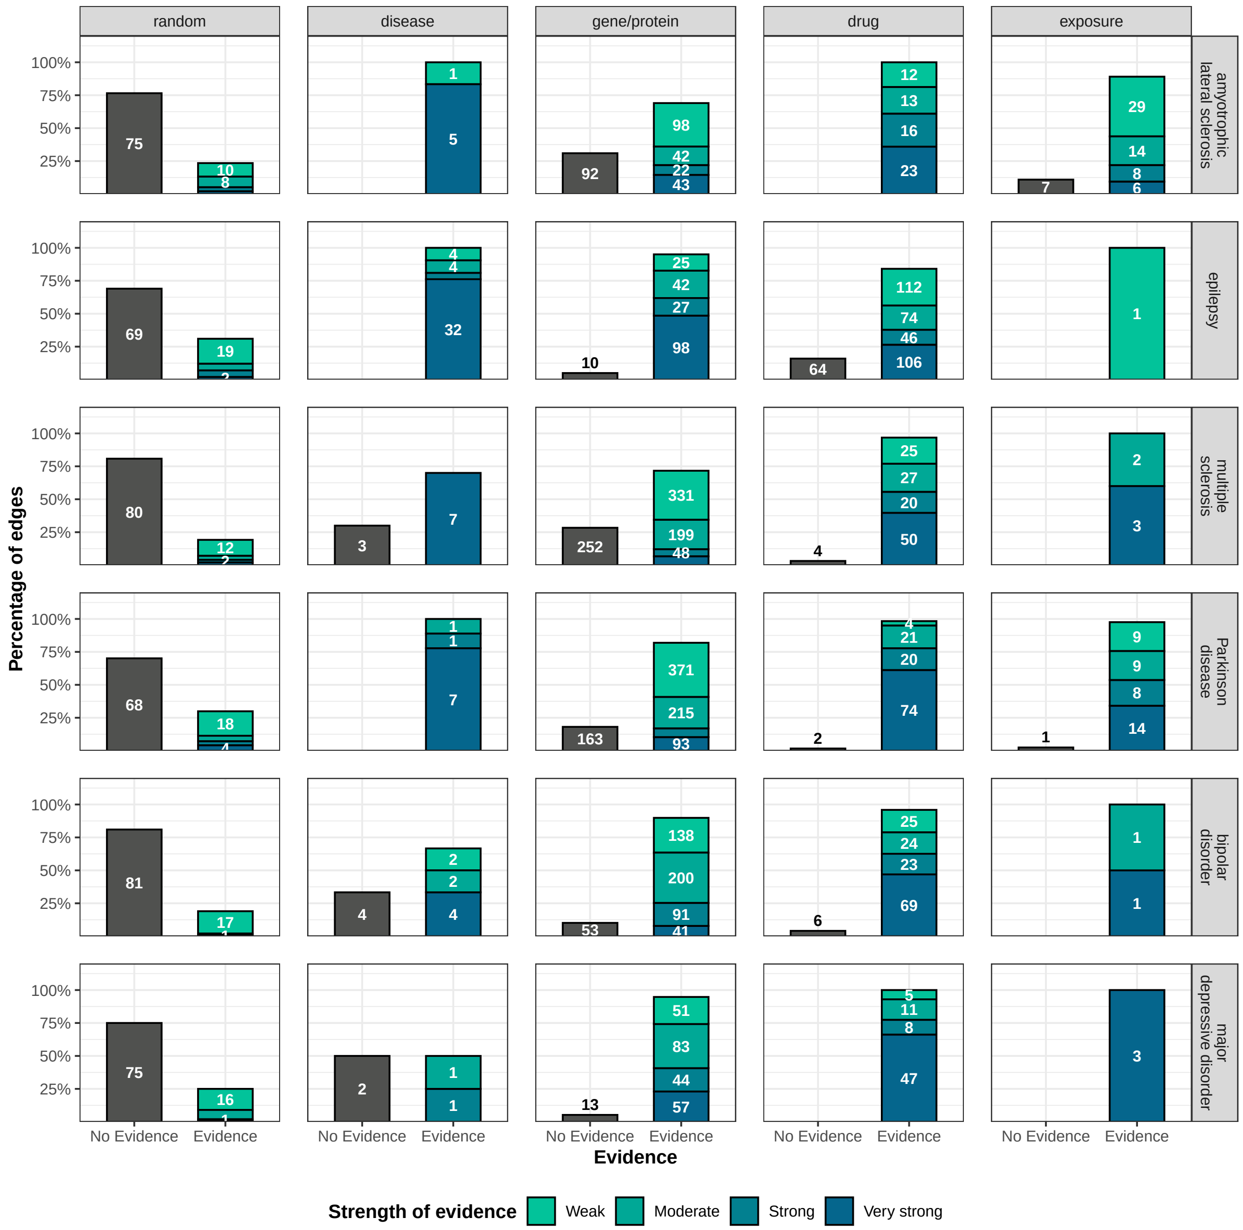


**Supplementary Figure 6: Disease edges in NEUROKG are supported by literature evidence retrieved by an AI agent.** PaperQA2, a frontier language-based generative AI agent that retrieves and reasons on information from the scientific literature [14], was used to assess the presence or absence of evidence supporting edges of type `(disease, disease)`, `(disease, gene/protein)`, `(disease, drug)`, or `(disease, exposure)` incident on six neurological diseases in NEUROKG. The PaperQA2 AI agent identified evidence in the scientific literature to support 83.87% of edges ($n = 3,514$). By contrast, 75.54% ($n = 448$) of randomly sampled non-edges were not supported by any evidence (leftmost column). The height of bars represents group-wise percentages, while numeric labels represent edge count.

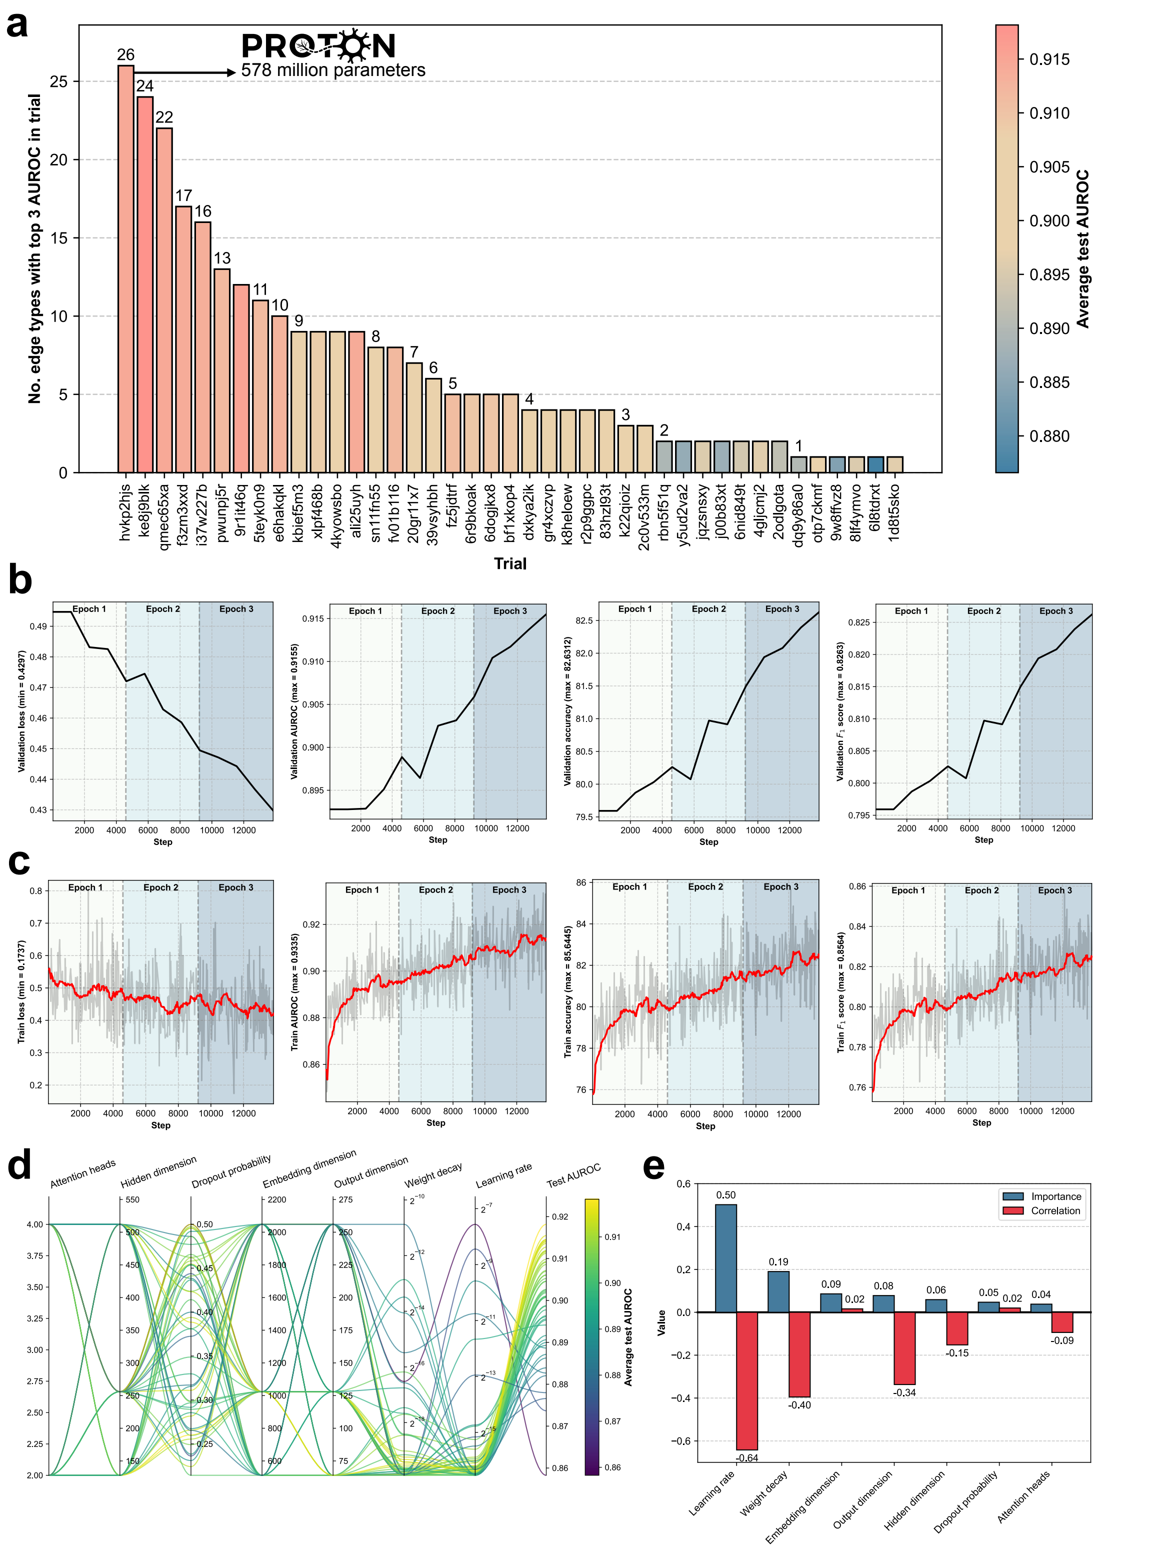


**Supplementary Figure 7: Performance across 55 hyperparameter optimization trials to design the PROTON architecture. (a)** For each trial, the number of edge types in which that trial is among the top 3 best-performing trials (based on edge-type-specific test AUROC) is shown. (cont.)

**Supplementary Figure 7:** (cont.) PROTON (trial ID: `hvkp2hjs`) is best performing in 26 edge types. **(b)** Validation loss, AUROC, accuracy, and $F_1$ score across three epochs of pre-training for a representative trial. **(c)** Pre-training loss, AUROC, accuracy, and $F_1$ score for a representative trial. Values are sampled for visualization. The rolling window average with a window size of 25 is shown in red. **(d)** Parallel coordinate plot of hyperparameter settings across trials. Trials are colored by test AUROC. **(e)** Importance of each hyperparameter with respect to test AUROC, as well as correlation with test AUROC.

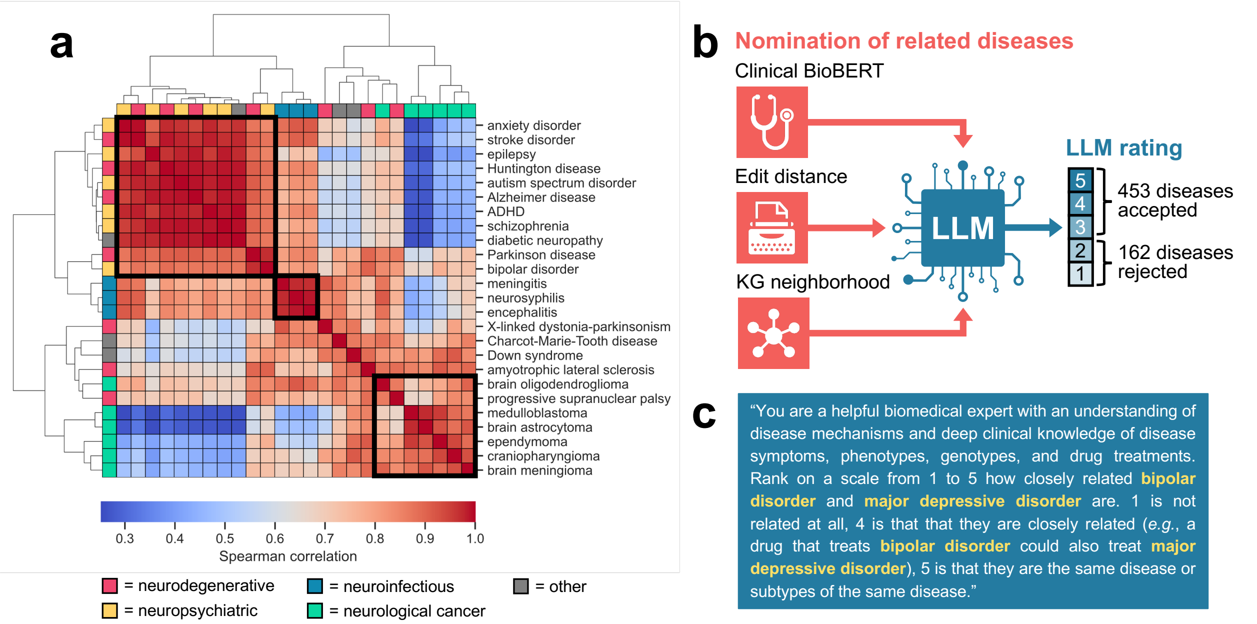


**Supplementary Figure 8: PROTON makes consistent predictions across related diseases. (a)** PROTON makes similar predictions for related diseases based on Spearman correlation of the 3,071 drugs that appear at rank $\leq 2,000$ in at least one of the 25 diseases. Diseases are grouped into neurodegenerative, neuropsychiatric, neuroinfectious, neurological cancer, and other categories. **(b)** The process of identifying diseases for inclusion in the disease-centric split is depicted. For each of 17 neurological diseases, related diseases were nominated for inclusion using Clinical BioBERT embedding similarity [29], Levenshtein edit distance between disease names, or one-hop neighborhood overlap in NEUROKG. Candidate diseases were reviewed and rated by GPT-4o, with diseases scoring $\geq 3$ included in the split. **(c)** An example of the prompt used for disease similarity rating; in this case, comparing bipolar disorder and major depressive disorder.

| Cell type | Total cells | Subtypes | Subclusters |
|---|---|---|---|
| **Neurons** | | | |
| Upper-layer intratelencephalic | 452,715 | 16 | 139 |
| Splatter | 273,703 | 90 | 1135 |
| CGE interneuron | 226,007 | 21 | 180 |
| MGE interneuron | 219,640 | 26 | 211 |
| Deep-layer intratelencephalic | 209,135 | 14 | 127 |
| Medium spiny neuron | 150,318 | 18 | 143 |
| Upper rhombic lip | 136,377 | 6 | 21 |
| Midbrain-derived inhibitory | 124,243 | 12 | 64 |
| Amygdala excitatory | 106,706 | 18 | 138 |
| Deep-layer corticothalamic and 6b | 77,365 | 17 | 116 |
| Thalamic excitatory | 75,529 | 17 | 109 |
| Hippocampal dentate gyrus | 67,245 | 7 | 26 |
| Hippocampal CA1-3 | 52,990 | 14 | 73 |
| Lower rhombic lip | 49,523 | 6 | 25 |
| LAMP5-LHX6 and Chandelier | 44,519 | 12 | 55 |
| Eccentric medium spiny neuron | 39,628 | 14 | 96 |
| Miscellaneous | 24,422 | 22 | 102 |
| Deep-layer near-projecting | 18,736 | 13 | 72 |
| Mammillary body | 14,205 | 9 | 37 |
| Cerebellar inhibitory | 13,974 | 10 | 38 |
| Hippocampal CA4 | 10,575 | 9 | 40 |
| **Non-neuronal cells** | | | |
| Oligodendrocyte | 489,306 | 8 | 24 |
| Astrocyte | 154,679 | 13 | 71 |
| Oligodendrocyte precursor | 105,640 | 5 | 19 |
| Microglia | 91,432 | 9 | 30 |
| Vascular | 9,792 | 11 | 41 |
| Fibroblast | 9,036 | 8 | 25 |
| Bergmann glia | 8,039 | 1 | 1 |
| Choroid plexus | 7,404 | 7 | 22 |
| Ependymal | 5,432 | 10 | 43 |
| Committed oligodendrocyte precursor | 4,538 | 7 | 21 |

**Supplementary Table 1: Neuronal and non-neuronal cell types in Siletti *et al.*** Cell type counts are shown after pre-processing and quality control analyses.

| Node type | Number of nodes | Average degree |
|---|---|---|
| gene/protein | 35,198 | 163.93 ± 157.85 |
| biological process | 27,668 | 8.70 ± 27.20 |
| disease | 22,201 | 28.42 ± 145.41 |
| effect/phenotype | 16,711 | 18.55 ± 81.27 |
| anatomy | 14,384 | 290.93 ± 2197.55 |
| molecular function | 11,228 | 8.71 ± 128.94 |
| drug | 8,160 | 370.45 ± 537.77 |
| cellular component | 4,054 | 22.81 ± 202.48 |
| cell subcluster | 3,244 | 50.52 ± 3.92 |
| pathway | 2,629 | 18.79 ± 29.59 |
| exposure | 860 | 12.80 ± 34.45 |
| cell cluster | 450 | 210.67 ± 11.14 |
| brain structure | 112 | 17.25 ± 11.59 |
| cell subtype | 68 | 595.12 ± 48.51 |
| cell type | 39 | 575.69 ± 325.95 |
| brain region | 14 | 8.00 ± 9.27 |

**Supplementary Table 2: Node types and statistics in NEUROKG.** Average degree is reported as mean ± SD.

| ID | Line | Cohort or study ID | Age | Sex | Diagnosis |
|---|---|---|---|---|---|
| CM2 | PSC-01-020 | Yankner/Tsai | 38 | M | Control |
| CM3 | MH0185983 | NRGR Study ID 163 | 29 | M | Control |
| CM4 | MH0185932 | NRGR Study ID 163 | 19 | M | Control |
| CF4 | MH0185863 | NRGR Study ID 163 | 36 | F | Control |
| BF1 | BD-220-5 | Yankner/Tsai | 49 | F | BD |
| BF3 | BD-12-33 | Yankner/Tsai | 35 | F | BD |
| BF4 | BD-193-3 | Yankner/Tsai | 32 | F | BD |
| BF5 | BD-PSC-01-002 | Yankner/Tsai | 46 | F | BD |
| BM4 | MH0185869 | NRGR Study ID 163 | 26 | M | BD |

**Supplementary Table 3: iPSC lines used to generate cerebral brain organoids.** iPSC lines in this study were obtained from Meyer *et al.* [30].

| ICD-10 code | Description |
| --- | --- |
| **Alzheimer's disease and related dementias (ADRD)** | |
| F01.50 | Vascular dementia without behavioral disturbance |
| F01.51 | Vascular dementia with behavioral disturbance |
| F02.80 | Dementia in other diseases classified elsewhere without behavioral disturbance |
| F02.81 | Dementia in other diseases classified elsewhere with behavioral disturbance |
| F03.90 | Unspecified dementia, unspecified severity, without behavioral disturbance, psychotic disturbance, mood disturbance, and anxiety |
| F03.91 | Unspecified dementia, unspecified severity, with behavioral disturbance |
| F04 | Amnestic disorder |
| G30.0 | Alzheimer's disease with early onset |
| G30.1 | Alzheimer's disease with late onset |
| G30.8 | Other Alzheimer's disease |
| G30.9 | Alzheimer's disease, unspecified |
| G31.0 | Frontotemporal dementia |
| G31.01 | Pick's disease |
| G31.09 | Other frontotemporal neurocognitive disorder |
| G31.1 | Senile degeneration of brain, not elsewhere classified |
| G31.8 | Other specified degenerative disease of nervous system |
| G31.83 | Neurocognitive disorder with Lewy bodies |
| G31.84 | Mild cognitive impairment of uncertain or unknown etiology |
| G31.85 | Corticobasal degeneration |
| G31.89 | Other specified degenerative disease of nervous system |
| G31.9 | Degenerative disease of nervous system, unspecified |
| R41.81 | Age-related cognitive decline |
| **Type 2 diabetes mellitus** | |
| E11* | Type 2 diabetes mellitus, including all subcategories |
| **Wet age-related macular degeneration** | |
| H35.32 | Exudative age-related macular degeneration |
| **Hypercholesterolemia** | |
| E78.00 | Pure hypercholesterolemia, unspecified |
| **Hyperlipidemia** | |
| E78* | Disorders of lipoprotein metabolism and other lipidemias* |
| **Hypertension** | |
| I10* | Essential hypertension* |

**Supplementary Table 4: ICD-10 diagnosis codes.** Diagnosis codes were used to define dementia and non-dementia indications for emulated target trials. For hyperlipidemia and hypertension, ICD codes were further refined using SQL `LIKE` clauses to those containing the phrases "hyperlipidemia" or "hypertension," respectively. This step improved precision in cohort definitions (*e.g.*, by excluding secondary hypertensive disorders from the hypertension cohort).

| Sweep | AUROC | Accuracy | AP | $F_1$ score | Loss |
|---|---|---|---|---|---|
| **Training metrics** | | | | | |
| ke8j9blk | 0.9217 | 0.8271 | 0.9158 | 0.8271 | 0.6093 |
| 9r1it46q | 0.9133 | 0.8252 | 0.9059 | 0.8252 | 0.6645 |
| qmec65xa | 0.9189 | 0.8350 | 0.9104 | 0.8350 | 0.3970 |
| **hvkp2hjs** | 0.9129 | 0.8232 | 0.9064 | 0.8232 | 0.4939 |
| ali25uyh | 0.9103 | 0.8223 | 0.9068 | 0.8223 | 0.5563 |
| f3zm3xxd | 0.9115 | 0.8232 | 0.9049 | 0.8232 | 0.4369 |
| i37w227b | 0.9229 | 0.8311 | 0.9165 | 0.8311 | 0.2383 |
| e6hakqkl | 0.9089 | 0.8223 | 0.9001 | 0.8223 | 0.5751 |
| pwunpj5r | 0.9125 | 0.8223 | 0.9088 | 0.8223 | 0.3639 |
| fv01b116 | 0.9272 | 0.8350 | 0.9213 | 0.8350 | 0.3425 |
| **Validation metrics** | | | | | |
| ke8j9blk | 0.9179 | 0.8289 | 0.9115 | 0.8289 | 0.4291 |
| 9r1it46q | 0.9155 | 0.8263 | 0.9092 | 0.8263 | 0.4297 |
| qmec65xa | 0.9143 | 0.8244 | 0.9076 | 0.8244 | 0.4345 |
| **hvkp2hjs** | 0.9148 | 0.8228 | 0.9087 | 0.8228 | 0.4354 |
| ali25uyh | 0.9145 | 0.8225 | 0.9086 | 0.8225 | 0.4465 |
| f3zm3xxd | 0.9144 | 0.8237 | 0.9082 | 0.8237 | 0.4438 |
| i37w227b | 0.9136 | 0.8219 | 0.9072 | 0.8219 | 0.4370 |
| e6hakqkl | 0.9127 | 0.8214 | 0.9065 | 0.8214 | 0.4571 |
| pwunpj5r | 0.9119 | 0.8209 | 0.9051 | 0.8209 | 0.4329 |
| fv01b116 | 0.9116 | 0.8203 | 0.9056 | 0.8203 | 0.4519 |
| **Test metrics** | | | | | |
| ke8j9blk | 0.9182 | 0.8293 | 0.9118 | 0.8293 | 0.4291 |
| 9r1it46q | 0.9155 | 0.8265 | 0.9091 | 0.8265 | 0.4329 |
| qmec65xa | 0.9145 | 0.8246 | 0.9081 | 0.8246 | 0.4357 |
| **hvkp2hjs** | 0.9145 | 0.8223 | 0.9085 | 0.8223 | 0.4356 |
| ali25uyh | 0.9142 | 0.8222 | 0.9083 | 0.8222 | 0.4512 |
| f3zm3xxd | 0.9140 | 0.8235 | 0.9077 | 0.8235 | 0.4466 |
| i37w227b | 0.9136 | 0.8220 | 0.9073 | 0.8220 | 0.4348 |
| e6hakqkl | 0.9127 | 0.8215 | 0.9066 | 0.8215 | 0.4546 |
| pwunpj5r | 0.9119 | 0.8206 | 0.9051 | 0.8206 | 0.4395 |
| fv01b116 | 0.9118 | 0.8206 | 0.9059 | 0.8206 | 0.4505 |

**Supplementary Table 5: Pre-training metrics of top 10 hyperparameter optimization trials ranked by test AUROC.** The trial configuration with the final selected hyperparameters is shown in bold typeface.

# References


1. Healy, J. & McInnes, L. Uniform manifold approximation and projection. *Nature Reviews Methods Primers* **4,** 1–15. doi:10.1038/s43586-024-00363-x (2024).
2. McInnes, L., Healy, J., Saul, N. & Großberger, L. UMAP: Uniform Manifold Approximation and Projection. *Journal of Open Source Software* **3,** 861. doi:10.21105/joss.00861 (2018).
3. Pedregosa, F. *et al.* Scikit-learn: Machine Learning in Python. *Journal of Machine Learning Research* **12,** 2825–2830 (2011).
4. Vasilevsky, N. A. *et al. Mondo: Unifying diseases for the world, by the world* 2022. doi:10.1101/2022.04.13.22273750.
5. Shefchek, K. A. *et al.* The Monarch Initiative in 2019: an integrative data and analytic platform connecting phenotypes to genotypes across species. *Nucleic Acids Research* **48,** D704–D715. doi:10.1093/nar/gkz997 (2020).
6. Chari, T. & Pachter, L. The specious art of single-cell genomics. *PLOS Computational Biology* **19,** e1011288. doi:10.1371/journal.pcbi.1011288 (2023).
7. Weininger, D. SMILES, a chemical language and information system. *Journal of Chemical Information and Computer Sciences* **28,** 31–36. doi:10.1021/ci00057a005 (1988).
8. Kim, S. *et al.* PubChem 2025 update. *Nucleic Acids Research* **53,** D1516–D1525. doi:10.1093/nar/gkae1059 (2025).
9. Wishart, D. S. *et al.* DrugBank 5.0: a major update to the DrugBank database for 2018. *Nucleic Acids Research* **46,** D1074–D1082. doi:10.1093/nar/gkx1037 (2018).
10. Landrum, G. *et al. RDKit: Open-source cheminformatics.* 2022. doi:10.5281/zenodo.6483170.
11. Cereto-Massagué, A., Ojeda, M. J., Valls, C., Mulero, M., Garcia-Vallvé, S. & Pujadas, G. Molecular fingerprint similarity search in virtual screening. *Methods. Virtual Screening* **71,** 58–63. doi:10.1016/j.ymeth.2014.08.005 (2015).
12. Morgan, H. L. The Generation of a Unique Machine Description for Chemical Structures-a Technique Developed at Chemical Abstracts Service. *Journal of chemical documentation* **5,** 107–113 (1965).
13. OpenAI *et al. GPT-4o System Card* 2024. doi:10.48550/arXiv.2410.21276.
14. Skarlinski, M. D. *et al. Language agents achieve superhuman synthesis of scientific knowledge* 2024. doi:10.48550/arXiv.2409.13740.
15. Lála, J., O'Donoghue, O., Shtedritski, A., Cox, S., Rodriques, S. G. & White, A. D. *PaperQA: Retrieval-Augmented Generative Agent for Scientific Research* 2023. doi:10.48550/arXiv.2312.07559.
16. Lewis, P. *et al. Retrieval-Augmented Generation for Knowledge-Intensive NLP Tasks* in *Advances in Neural Information Processing Systems* **33** (Curran Associates, Inc., 2020), 9459–9474.
17. Sjöstedt, E. *et al.* An atlas of the protein-coding genes in the human, pig, and mouse brain. *Science* **367,** eaay5947. doi:10.1126/science.aay5947 (2020).

18. Mungall, C. J., Torniai, C., Gkoutos, G. V., Lewis, S. E. & Haendel, M. A. Uberon, an integrative multi-species anatomy ontology. *Genome Biology* **13,** R5. doi:10.1186/gb-2012-13-1-r5 (2012).

19. Haendel, M. A. *et al.* Unification of multi-species vertebrate anatomy ontologies for comparative biology in Uberon. *Journal of Biomedical Semantics* **5,** 21. doi:10.1186/2041-1480-5-21 (2014).

20. Chandak, P., Huang, K. & Zitnik, M. Building a knowledge graph to enable precision medicine. *Scientific Data* **10,** 67. doi:10.1038/s41597-023-01960-3 (2023).

21. Hu, W. *et al. Open graph benchmark: datasets for machine learning on graphs* in *Proceedings of the 34th International Conference on Neural Information Processing Systems* (Curran Associates Inc., Red Hook, NY, USA, 2020), 22118–22133.

22. Himmelstein, D. S. *et al.* Systematic integration of biomedical knowledge prioritizes drugs for repurposing. *eLife* **6** (ed Valencia, A.) e26726. doi:10.7554/eLife.26726 (2017).

23. Zheng, S. *et al.* PharmKG: a dedicated knowledge graph benchmark for bomedical data mining. *Briefings in Bioinformatics* **22,** bbaa344. doi:10.1093/bib/bbaa344 (2021).

24. Romano, J. D. *et al.* The Alzheimer's Knowledge Base: A Knowledge Graph for Alzheimer Disease Research. *Journal of Medical Internet Research* **26,** e46777 (2024).

25. Lyketsos, C. G. *et al.* Neuropsychiatric symptoms in Alzheimer's disease. *Alzheimer's & Dementia* **7,** 532–539. doi:10.1016/j.jalz.2011.05.2410 (2011).

26. Aarsland, D., Marsh, L. & Schrag, A. Neuropsychiatric symptoms in Parkinson's disease. *Movement Disorders* **24,** 2175–2186. doi:10.1002/mds.22589 (2009).

27. Ihara, M. & Saito, S. Drug Repositioning for Alzheimer's Disease: Finding Hidden Clues in Old Drugs. *Journal of Alzheimer's Disease* **74,** 1013–1028. doi:10.3233/JAD-200049 (2020).

28. Siletti, K. *et al.* Transcriptomic diversity of cell types across the adult human brain. *Science* **382,** eadd7046. doi:10.1126/science.add7046 (2023).

29. Alsentzer, E. *et al. Publicly Available Clinical BERT Embeddings* in *Proceedings of the 2nd Clinical Natural Language Processing Workshop* (Association for Computational Linguistics, Minneapolis, Minnesota, USA, 2019), 72–78.

30. Meyer, K. *et al.* Impaired neural stress resistance and loss of REST in bipolar disorder. *Molecular Psychiatry* **29,** 153–164. doi:10.1038/s41380-023-02313-7 (2024).
